# Supplementary material for: Trustworthy FinAInce: Unpacking How AI-Mediated Financial Advice is Judged
Source: arXiv:2609.20989 source file (2026-09-21)
Supplement: Supplementary file 1 [file 8appendix.tex]

\setcounter{table}{0}
\renewcommand{\thetable}{A\arabic{table}}


\newpage
\input{tables/1_participant_demographics}

\input{tables/2_decision_context_definitions}

\input{tables/3_scenario_operationalization}





\section{Stimulus Construction Details with Example}
\label{app:stimulusConstruction}

To construct ecologically valid financial advice stimuli for the scenarios, we adopt an \textit{iterative} and \textit{semi-structured} generation pipeline that combines manual drafting, example-based inspiration, and LLM-assisted refinements. \textit{The primary aim of this design was to mimic how advice is communicated in the real world through the sources of interest: online community forums, certified financial planners, and financial AI assistants, while simultaneously controlling the financial content and recommendations across all versions.}

\begin{enumerate}
    \item For each scenario, we first reviewed relevant discussions from online forums such as Reddit (r/personalfinance, r/investment, r/bogleheads), financial advisory blogs, articles, and videos (SmartAssets, Yahoo Finance, The College Investor, Bogleheads.org), general financial principles, as well as responses from AI chatbots such as ChatGPT and Claude. This helped us observe and understand plausible financial strategies, common heuristics, and reasoning patterns, thereby improving ecological validity. 
    \item We then construct a core decision backbone comprising relevant financial principles, numerical values, mathematical calculations, and the overall direction of the recommendation. This backbone served as the fundamental starting point for all three versions of the advice, ensuring that they all reflect the same financial reasoning and constraints.
    \item Finally, we model this core decision backbone into three advice versions:
    \begin{itemize}
        \item \textbf{Online Community Style}: Online community-style responses were initially manually drafted based on recurring communication patterns observed in financial discussion forums and subsequently refined using an LLM for consistency, readability, and length.
        \item \textbf{Expert Style}: Expert-style responses were produced through an iterative few-shot rewriting process in which public-facing financial-planning Q\&A examples (like \textit{Smart Assets} Q\&A forum and \textit{Yahoo Finance} Forum) were used to guide the transformation of each common decision backbone. The generation process targeted the stylistic characteristics summarized in Table~\ref{tab:advice_style_operationalization}. 
        \item \textbf{AI Style}: AI-style responses were generated using a constraint-based prompting approach, in which we provided the online community response and the corresponding decision backbone as the input. The LLM was specifically instructed to retain the same financial facts, rules, and strategic direction when rewriting the response. The generation process had these explicit constraints regarding use of personal experience, introduction of new numbers, assumptions, or calculations, neutral analytical tone and clear and concise sentence structure. Complete prompt can be found in~\ref{app:ai_generation_prompt}

% Because stimulus development was iterative, the exact conversational prompts used during early construction were not retained.
    \end{itemize}

    \item \textbf{Content-Parity Check.} Within each scenario, the three advice versions preserved the same core financial facts, recommendation direction, and substantive reasoning. We manually reviewed the stimuli to ensure that stylistic rewriting did not introduce new financial assumptions, contradictory calculations, or substantive changes in the recommended strategy. Advice length was also controlled within scenarios, with versions generally differing by no more than approximately ten words and ranging from roughly 140--190 words depending on scenario complexity. All advice was displayed using the same visual format; we intentionally did not reproduce platform-specific interfaces such as chatbot windows, advisory webpages, or Reddit threads, thereby avoiding visual-interface cues as an additional source manipulation. Full stimuli are provided in the supplementary material. 

\end{enumerate}



\subsection{Source-Specific Communication-Style Operationalization}
\input{tables/4_advicestyleOperationalization}

\FloatBarrier

\subsection{Prompt for generating AI-style Advice}
\label{app:ai_generation_prompt}

The following prompt was used to generate the Financial AI Assistant responses.

\begin{quote}
\small

\textbf{Role.}
You are a neutral AI financial assistant.

\medskip

You need to generate advice for the given scenario. You have been provided
with a response from a top-rated comment in an online community forum and a
decision backbone. Your goal is to generate a response that maintains
information parity regarding financial facts, rules, strategy, and the
direction of the decision. The response should be distinctly AI-generated.

\medskip

\textbf{Constraints.}
\begin{itemize}
    \item Do not reference personal experience.
    \item Do not use storytelling language.
    \item Do not use emotional validation.
    \item Do not invent new assumptions.
    \item Do not introduce numbers that are not in both responses and the scenario.
    \item Do not introduce new calculations.
    \item Use a neutral, analytical tone.
    \item Do not repeat facts unnecessarily.
    \item Do not use complex sentences.
    \item Address the protagonist as ``you.''
    \item Write exactly three paragraphs. The paragraphs can vary in length as required by the scenario.
    \item Word limit: \textit{average length of the OC and Expert responses $\pm$ 10 words}.
    \item The response should be logical.
    \item Assume that the protagonist has experience with personal finance but is not an expert.
\end{itemize}

\textbf{Structure.}

\medskip

\textit{Paragraph 1:} Very briefly restate the financial situation and
quantify the financial difference using the provided numbers to establish
the trade-off or primary concern at hand.

\medskip

\textit{Paragraph 2:} Evaluate financial stability and risk exposure based
only on the income, savings, expenses, and debt mentioned. Use the relevant
rules or heuristics provided to explain the position.

\medskip

\textit{Paragraph 3:} Provide balanced conditional reasoning using
``If\ldots then\ldots'' framing and end with a sustainability-focused
consideration.

\medskip

\textbf{Inputs.}

\begin{itemize}
    \item \textit{[Scenario]}
    \item \textit{[Decision Backbone]}
    \item \textit{[Online Community Response]}
\end{itemize}

\end{quote}

\FloatBarrier

\subsection{Annotated Stimulus Example}
% ----------------------------------------------------------------------------
% 5. ANNOTATED STIMULUS EXAMPLE
% ----------------------------------------------------------------------------

% Figure: Controlled advice-style construction, page 1
\begin{figure*}[p]
    \centering
    \makebox[\textwidth][c]{%
        \includegraphics[
            page=1,
            width=1.06\textwidth,
            height=0.88\textheight,
            keepaspectratio,
            trim=10mm 16mm 8mm 14mm,
            clip
        ]{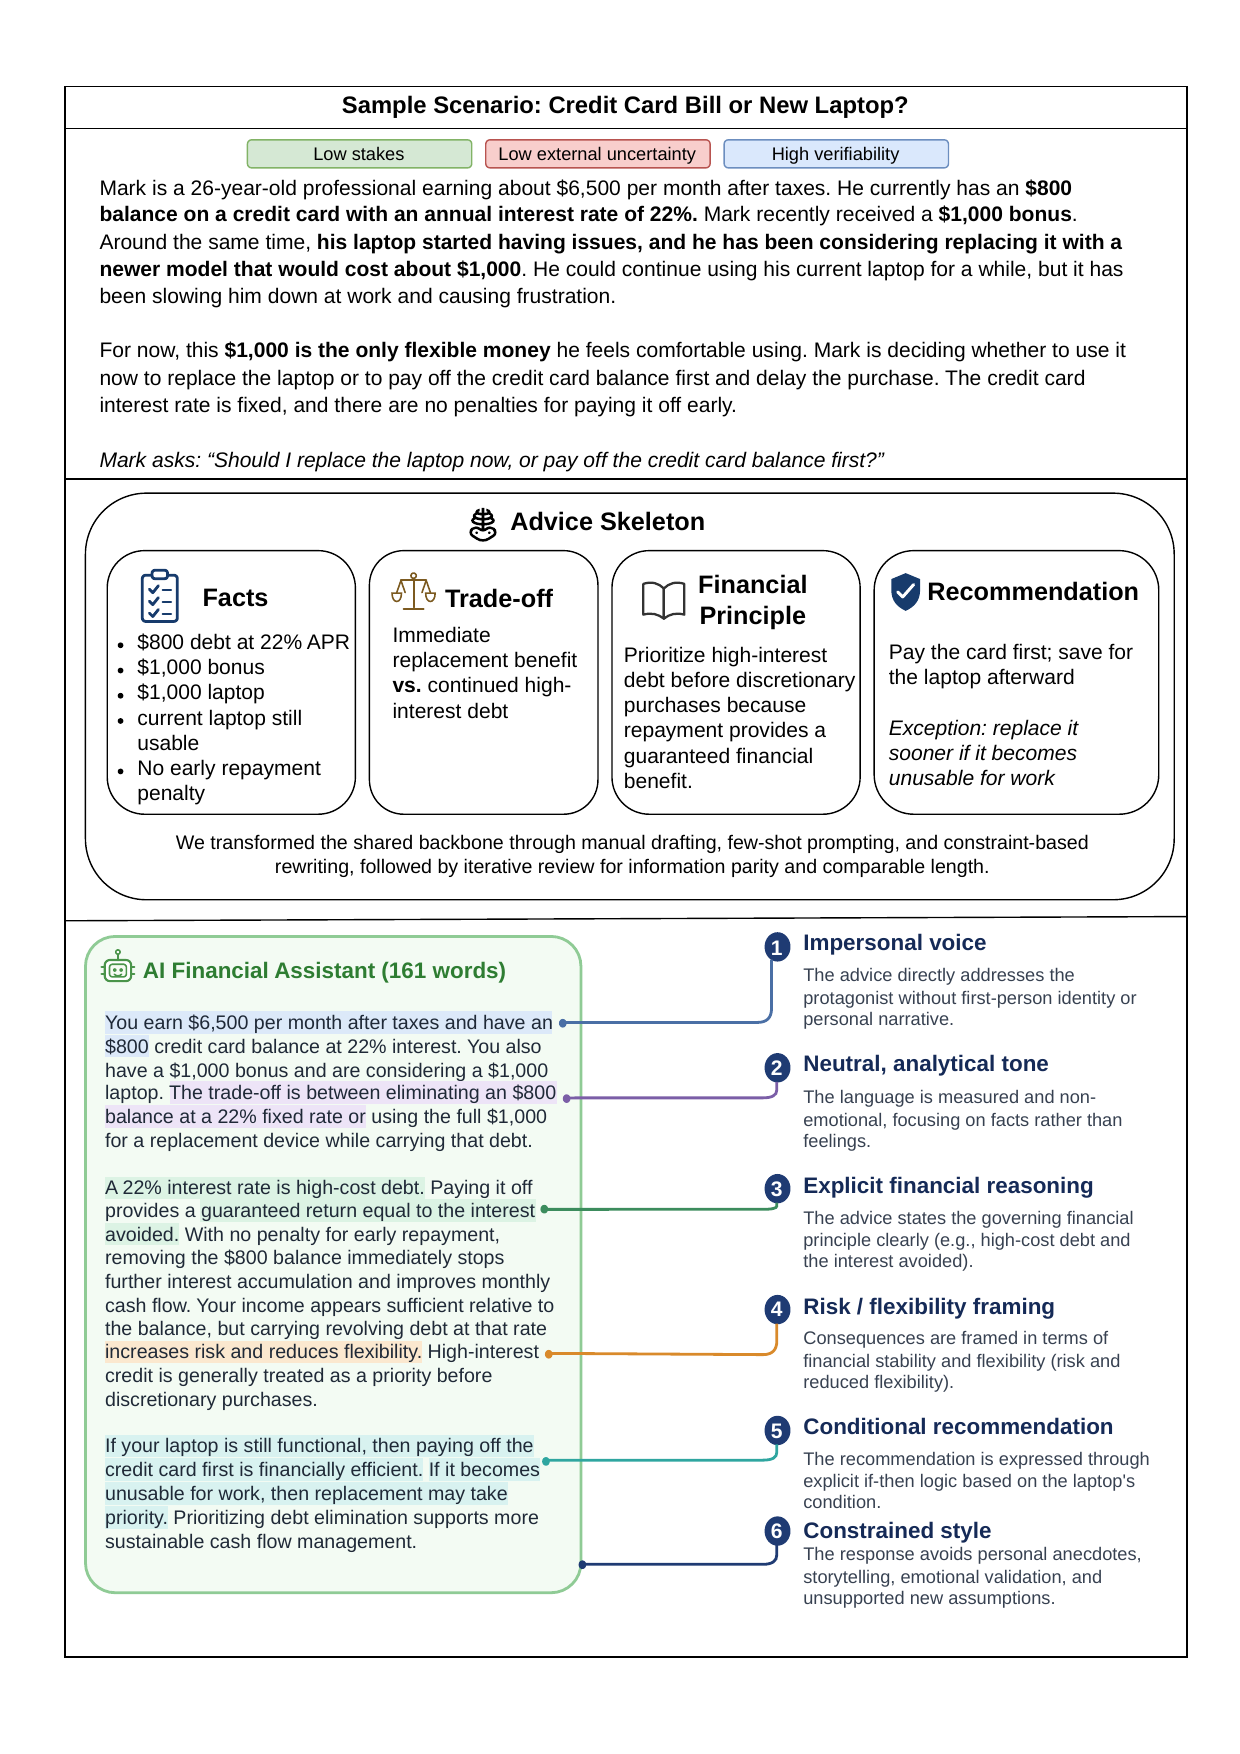}%
    }
    \Description{Page one of an annotated stimulus example. The credit-card-versus-laptop scenario is followed by a shared advice skeleton that lists the facts, trade-offs, financial principle, recommendation, and exception. A complete AI Financial Assistant response is highlighted and linked to numbered annotations identifying its impersonal voice, neutral analytical tone, explicit reasoning, risk framing, conditional recommendation, and constrained style.}

    \caption{
    \textbf{Controlled construction of source-specific advice styles.}
    A shared decision skeleton preserves the financial facts, governing
    principle, trade-off, recommendation direction, and boundary condition
    across all three responses. The same substantive backbone is rendered
    using the source-specific communication characteristics of an
    \emph{AI Financial Assistant}, a \emph{Certified Financial Planner}, and
    an \emph{Online Community Forum}. Highlighted passages and numbered
    annotations identify the voice, tone, framing, reasoning presentation,
    and discourse structure operationalized in each condition. Page one
    presents the financial scenario, common advice skeleton, and annotated
    AI Financial Assistant response.
    }
    \label{fig:annotated_advice_styles}
\end{figure*}

% Figure: Controlled advice-style construction, page 2 (continued)
\begin{figure*}[p]
    \ContinuedFloat
    \centering
    \makebox[\textwidth][c]{%
        \includegraphics[
            page=2,
            width=1.06\textwidth,
            height=0.93\textheight,
            keepaspectratio,
            trim=10mm 30mm 10mm 7mm,
            clip
        ]{figures/2_advice_example.drawio.pdf}%
    }
    \Description{Page two of the annotated stimulus example. Complete Certified Financial Planner and Online Community Forum responses are highlighted and linked to numbered annotations. The planner response illustrates quantified professional framing, restrained first-person authority, principle-based reasoning, actionable guidance, and long-term planning, while the community response illustrates an emphatic opening, conversational tone, personal experience, anecdotal reasoning, direct practical advice, and an emotional closing.}

    \caption[]{
    \textbf{Controlled construction of source-specific advice styles
    (continued).}
    Annotated Certified Financial Planner and Online Community Forum
    responses generated from the same substantive advice skeleton.
    }
\end{figure*}


\begin{figure*}[t]
    \centering
    \includegraphics[
         width=0.90\textwidth,
        trim={20bp 360bp 30bp 30bp},
        clip
    ]{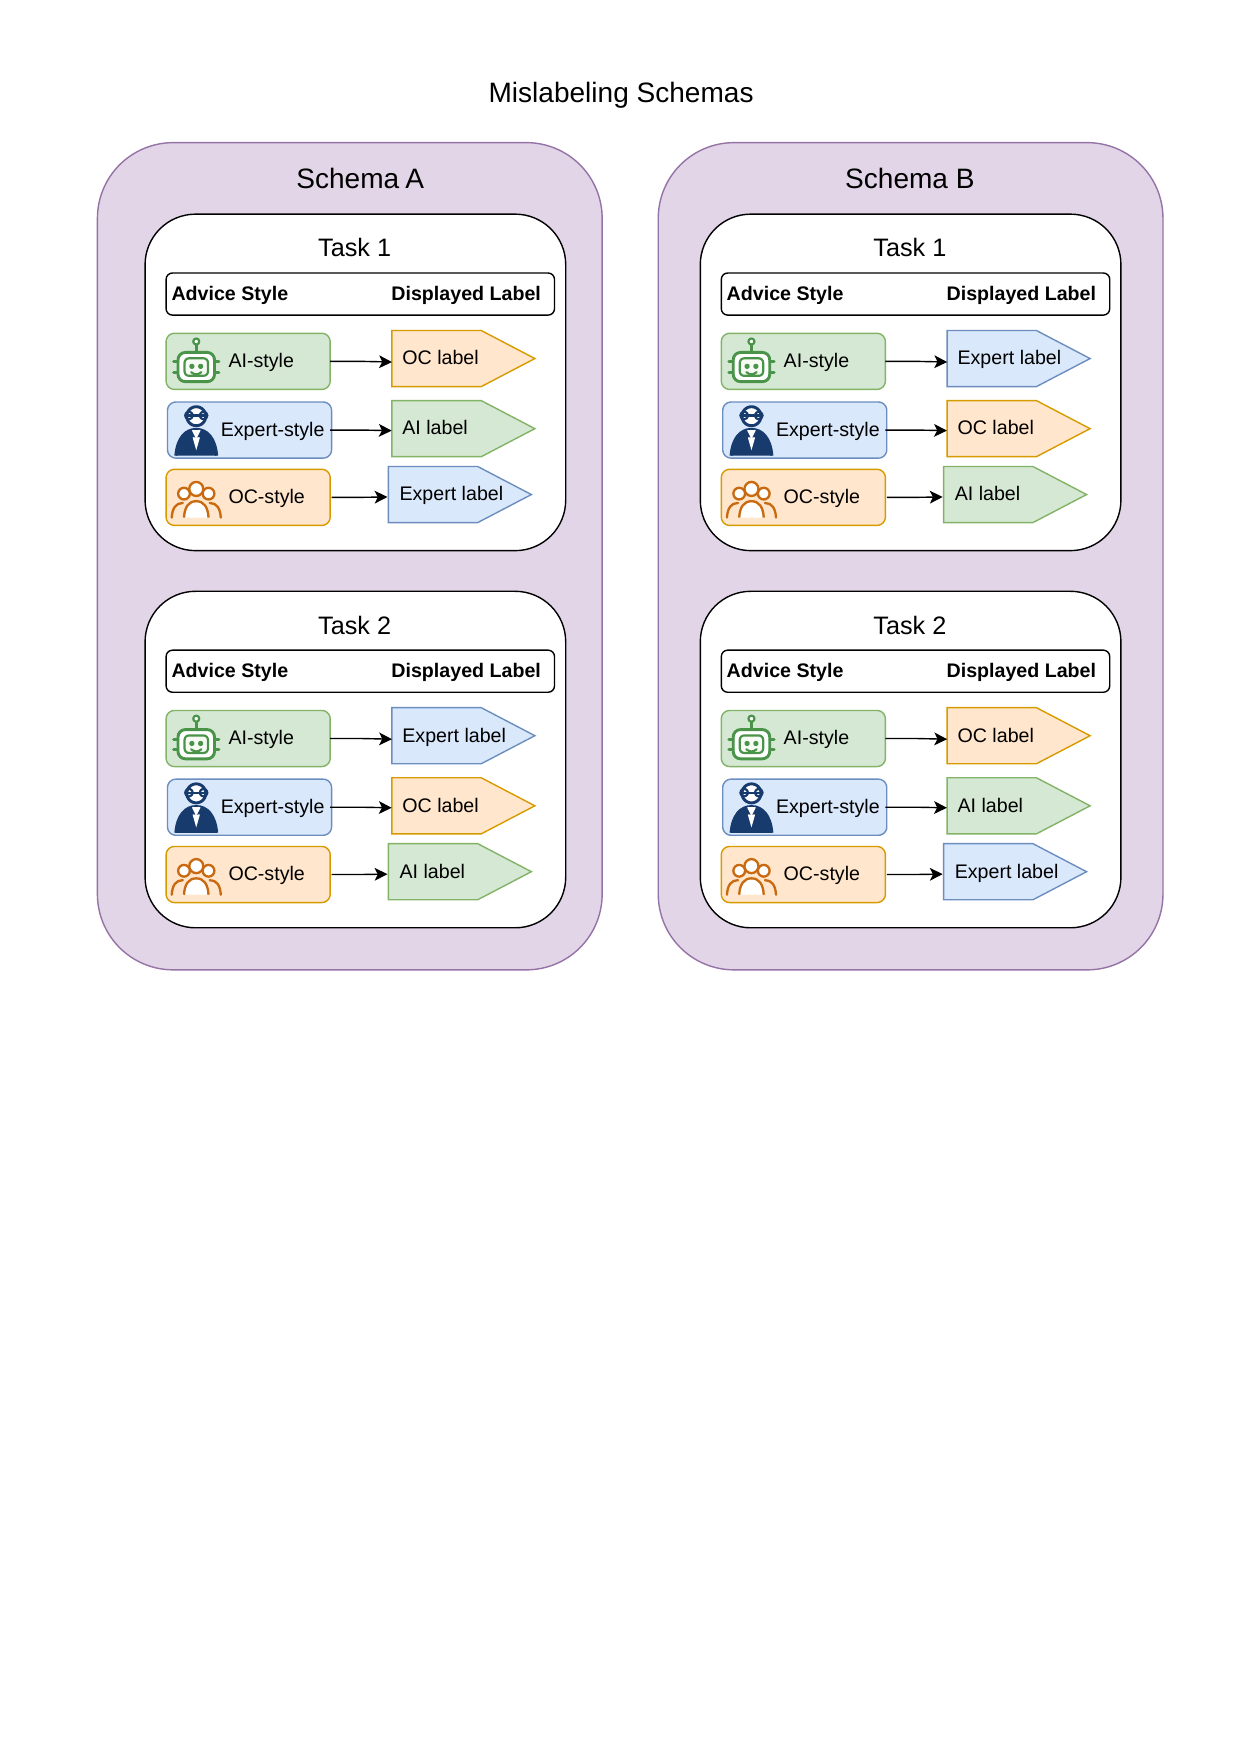}
\Description{
Two diagrams show the counterbalanced mislabeling schemas used across
the two experimental tasks. In Schema~A, Task~1 displays AI advice with
an OC label, Expert advice with an AI label, and OC advice with an Expert
label. In Task~2, AI advice is displayed with an Expert label, Expert
advice with an OC label, and OC advice with an AI label. Schema~B reverses
these mappings across tasks: Task~1 uses the Expert, OC, and AI labels
for AI, Expert, and OC advice, respectively, while Task~2 uses the OC,
AI, and Expert labels, respectively. In all cases, no advice style is
paired with its corresponding source label.
}

\caption{
Counterbalanced mislabeling schemas used across the two experimental
tasks. Participants in the mislabeled arm were assigned to one of two
label-swap schemas. In Schema~A, AI, Expert, and OC advice were displayed
with OC, AI, and Expert labels, respectively, in Task~1, and with Expert,
OC, and AI labels, respectively, in Task~2. Schema~B reversed these
mappings across tasks. Thus, no advice style was paired with its
corresponding source label in the \textit{mislabeled} condition, while
the counterbalancing varied which incorrect label each advice style
received across tasks.
}
    \label{fig:mislabeling_schemas}
\end{figure*}




\input{tables/5_evaluationItems}




\begin{figure*}[t]
    \centering
    \includegraphics[width=\linewidth]{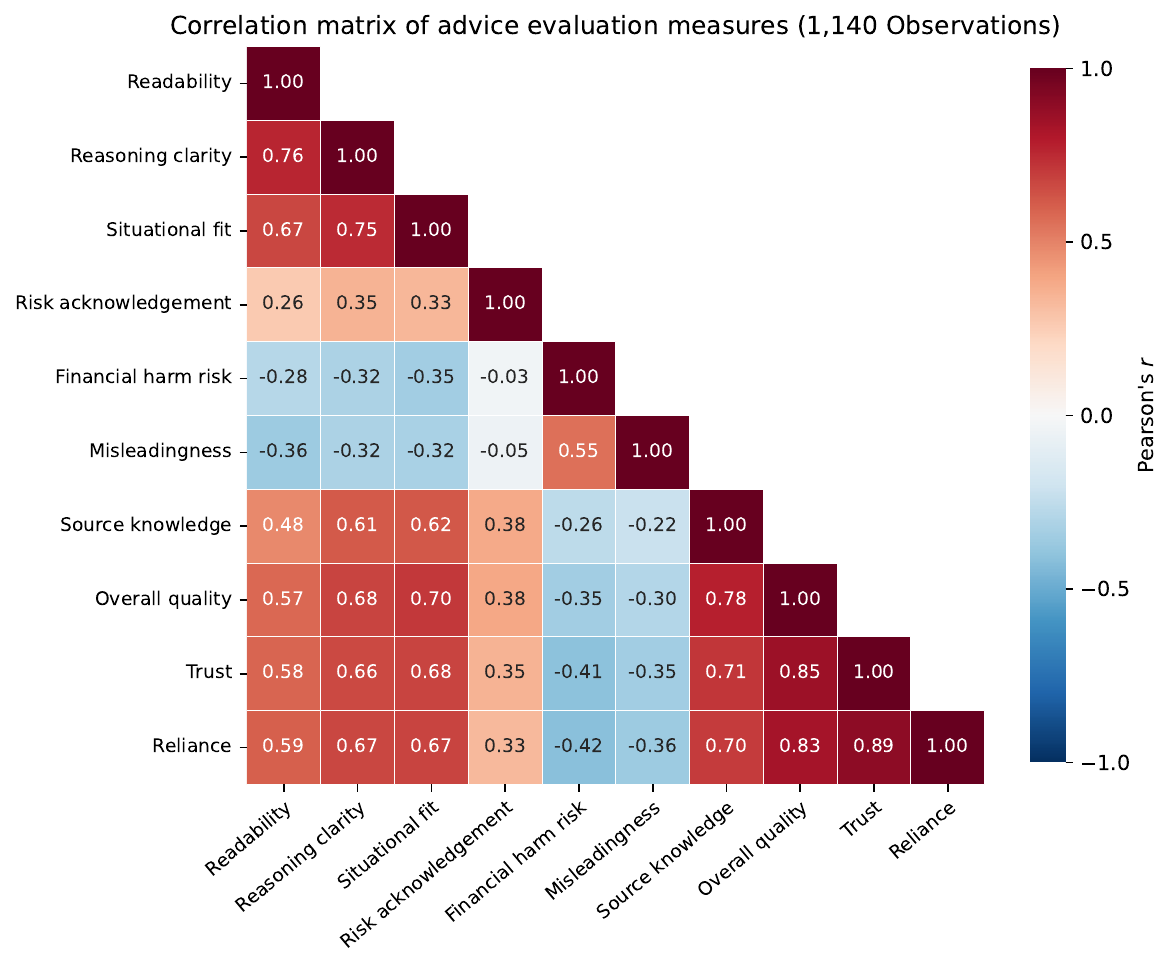}
    \caption{Pairwise correlations among advice evaluation measures. 
    Values indicate Pearson's $r$.}
    \Description{Lower-triangular correlation matrix showing pairwise Pearson correlations among readability, reasoning clarity, situational fit, risk acknowledgment, financial harm risk, misleadingness, source knowledge, overall quality, trust, and reliance.}
    \label{fig:correlation_matrix}
\end{figure*}

\input{tables/11_regression_formulas}
\input{tables/12_full_appraisal}
\input{tables/13_full_downstream}

\input{tables/15_full_reliance_bootstrap}
\input{tables/16_full_trust_bootstrap}
\input{tables/19_simple_effects_labels_styles}

\input{tables/17_Contrast_tables}

% \input{tables/21_trust_full_moderator}
% \input{tables/22_reliance_full_moderator}

\input{tables/23_individualmoderators}
\input{tables/24_equations_ind_moderators}
\input{tables/32_ind_moderators_vs_appraisals_full}
\input{tables/26_decisionContext_equations}

\input{tables/27_robustness_1}
\input{tables/28_robustness_2}
\input{tables/29_robustness_3}
\input{tables/30_robustness_4}


\input{tables/34_validation_appendix}

\input{tables/36_ranking_supplementary}
