# Supplementary material for: Trustworthy FinAInce: Unpacking How AI-Mediated Financial Advice is Judged
Source: arXiv:2609.20989 source file (2026-09-21)
Supplement: Supplementary file 3 [file scratch_supplementary.tex]

\subsection{Outcome Dimensionality \& Variable Construction}
The 10 advice evaluation outcomes were designed to capture complementary judgments rather than a single psychometric scale; hence, we first examined their empirical dimensionality. To avoid treating repeated evaluations from the same participant as independent observations, we averaged each item across the four advice evaluations completed by each participant and conducted an exploratory factor analysis on the resulting participant-level data (N = $285$). We used minimum residual (MINRES) extraction with oblimin rotation (\autoref{tab:efa_parallel}). The first three eigenvalues were $6.020$, $1.423$, and $0.706$. Horn's parallel analysis with 10,000 simulated datasets supported retaining two factors: the first two observed eigenvalues exceeded their corresponding 95th-percentile random eigenvalues ($1.390$ and $1.271$), whereas the third did not ($0.706$ vs. $1.187$). We interpret the retained structure through a broad positive evaluation dimension, including \textit{readability, reasoning clarity, situational fit, risk acknowledgment, perceived source knowledge, overall quality, trust}, and \textit{reliance}; and a second dimension defined primarily by \textit{perceived financial harm} and \textit{misleadingness}.

These results indicate that positive evaluation items largely move together rather than forming different empirical scales. Hence, we use factor analysis to characterize the overall structure of the ratings, while retaining theoretically meaningful distinctions among them. The Information Adoption Model (IAM) identifies \textit{argument quality} and \textit{source credibility} as key antecedents of perceived information usefulness and subsequent information adoption~\cite{sussmanInformationalInfluenceOrganizations2003},
while recent work applying IAM to financial AI additionally highlights
trust and perceived risk in the adoption process~\cite{ioannouRoleExplainabilityAIDriven2026}.
In our setting, message-level appraisals—readability, reasoning clarity, and situational fit—were averaged into a \textit{Message Appraisal} index ($\alpha=.887$) that captures properties related to argument quality, while perceived source knowledge was retained separately as a source-credibility judgment. Financial-harm risk and misleadingness were averaged into a \textit{Safety Concern} index ($\alpha=.712$; inter-item $r=.55$), with higher values indicating greater perceived concern, and risk acknowledgment was retained as an additional finance-relevant evaluation (Table~\ref{tab:composite_reliability}). Overall quality, trust, and reliance were retained separately as downstream judgments; distinguishing trust from reliance is also consistent with prior work on appropriate reliance in automation~\cite{leeTrustAutomationDesigning2004}.




\subsection{How Style and Source Labels Travel Through the Evaluation Pathway}
\label{sec:pathway_decomposition}

% \koustuv{This section I would move to the Appendix}

We next examined how communication style and displayed source labels
were associated with Reliance through the four intermediate appraisals.
We decomposed these associations into pathways through Message Appraisal,
Risk Acknowledgment, Safety Concern, and Source Knowledge, using
2,000 participant-level bootstrap samples to estimate 95\% confidence
intervals. These evaluations were measured within the same task; hence,
we interpret these results as statistical pathway decompositions rather
than causal mediation effects.

For \textbf{Expert-style advice relative to AI-style advice}, the total
appraisal-carried pathway to Reliance was positive
($\beta=.210$, 95\% CI $[.115,.309]$).
The largest contribution came through Message Appraisal
($\beta=.114$, 95\% CI $[.069,.166]$), with additional contributions
through lower Safety Concern
($\beta=.043$, 95\% CI $[.023,.068]$)
and greater Source Knowledge
($\beta=.055$, 95\% CI $[.009,.106]$).
In contrast, \textbf{OC-style advice} showed competing pathways:
it benefited through Message Appraisal
($\beta=.076$, 95\% CI $[.033,.123]$)
and lower Safety Concern
($\beta=.022$, 95\% CI $[.003,.045]$),
but was disadvantaged through lower Source Knowledge
($\beta=-.068$, 95\% CI $[-.129,-.014]$).
These opposing pathways largely canceled out, producing little net
appraisal-carried difference in Reliance
($\beta=.023$, 95\% CI $[-.083,.129]$).

Displayed source labels showed a different pattern.
An \textbf{Expert label}, relative to no label, had a positive total
appraisal-carried pathway
($\beta=.179$, 95\% CI $[.032,.325]$),
with the largest contribution through Source Knowledge
($\beta=.088$, 95\% CI $[.014,.164]$) followed by Message Appraisal ($\beta=.064$, 95\% CI $[.001,.129]$).
In comparison, we found no clear overall appraisal-carried pathway for
AI labels or OC labels relative to no label
(Table~\ref{tab:pathway_decomposition}).

Finally, we compared whether communication style and source labels placed
different relative weight on Message Appraisal versus Source Knowledge.
For Expert advice, communication style was more strongly associated with
the Message pathway than the corresponding Expert label
(contrast-of-contrasts: $\Delta\Delta=.081$,
95\% CI $[.014,.148]$).
The same pattern appeared for OC advice
($\Delta\Delta=.124$, 95\% CI $[.045,.212]$).
Together, these results suggest that \textbf{communication style operates
relatively more through evaluations of the message itself, whereas source
labels shift evaluation relatively toward perceptions of source
credibility}. A parallel analysis terminating at Trust showed the same
overall pattern (Table~\ref{tab:trust_pathways}).

\input{tables/14_bootstrap_table}
\input{tables/17_Contrast_tables}



\subsection{Do Source Labels Alter the Effects of Advice Style?}

We next tested whether the effect of the underlying communication style
depended on the source label displayed with the advice. For each outcome,
we compared the additive mixed-effects model to a model including the
\textit{Advice Style} $\times$ \textit{Displayed Label} interaction using a likelihood-ratio test. Adding the six interaction terms did not improve model fit for any of the
seven outcomes: Message Appraisal
($\chi^2(6)=3.71$, $p=.716$), Risk Acknowledgement
($\chi^2(6)=7.32$, $p=.293$), Safety Concern
($\chi^2(6)=2.20$, $p=.901$), perceived Source Knowledge
($\chi^2(6)=3.29$, $p=.772$), Overall Quality
($\chi^2(6)=4.83$, $p=.566$), Trust
($\chi^2(6)=1.48$, $p=.961$), or Reliance
($\chi^2(6)=2.17$, $p=.904$)
(Table~\ref{tab:style-label-interactions}). Thus, although communication
style and displayed attribution independently shaped several evaluations,
we found little evidence that the effect of one systematically depended on
the other.

We also examined simple contrasts within each style and label condition
(Appendix Tables~\ref{tab:label-within-style-matrix} and
\ref{tab:style-within-label-matrix}). Several style differences remained
detectable within particular labels; for example, Expert-style advice
received higher Message Appraisal than AI-style advice when unlabeled
($\beta=.390$, $p_{\mathrm{FDR}}=.001$) and when displayed with an Expert
label ($\beta=.493$, $p_{\mathrm{FDR}}=.006$). However, there was no
evidence that these differences changed systematically across labels.
Likewise, no label-within-style contrast remained significant after
false-discovery-rate (FDR) correction. \textbf{Taken together, these results support treating communication style and displayed attribution as largely additive rather
than interactive effects.}

However, such within-label
differences do not imply that the style difference itself changed across
labels, and the omnibus interaction tests above provided no evidence for
such moderation. Similarly, although several label-within-style contrasts
were nominally significant before correction, none survived
within-outcome false-discovery-rate correction. We therefore retain the
more parsimonious additive representation of communication style and
displayed attribution in the subsequent evaluation-pathway analyses.

\input{tables/18_likelihood_ratio_test}




\subsection{Individual Differences in Trust Formation and Reliance}
\label{sec:individual-differences}
\koustuv{move this to appendix.}

We next examined whether participant characteristics were associated with
overall Trust and Reliance, and whether they altered how advice evaluations
translated into these downstream judgments. We considered seven
participant-level characteristics: General AI Trust, AI Literacy, Human
Trust Propensity (HTP), Objective Financial Literacy, Self-rated Financial
Literacy, Risk Tolerance, and prior AI Use for Finance. Continuous
moderators were standardized prior to analysis. All models included
participant random intercepts and controlled for communication style,
displayed source label, decision-context characteristics, and scenario
familiarity. Benjamini--Hochberg false-discovery-rate (FDR) correction was
applied within each prespecified family of moderator tests.



\paragraph{Individual differences in overall Trust.}
We first examined whether participant characteristics were associated with
the overall level of Trust. All seven characteristics were entered
simultaneously in an upstream model containing the experimental and
decision-context controls. General AI Trust was the only characteristic
showing a robust association with Trust
($\beta=.202$, $p_{\mathrm{FDR}}<.001$). Participants higher in General AI
Trust therefore tended to report greater Trust in the advice overall.
After additionally accounting for Message Appraisal, Risk Acknowledgment,
Safety Concern, Source Knowledge, and Overall Quality, this association
was substantially attenuated
($\beta=.046$, $p_{\mathrm{FDR}}=.109$).
No other participant characteristic showed a robust main association with
Trust after FDR correction.

\paragraph{Individual differences in initial appraisals.}
We additionally examined whether participant characteristics were associated
with the initial evaluations participants formed about the advice. Several
characteristics showed distinct appraisal-level associations
(Table~\ref{tab:individual-appraisal-main}). Greater AI Literacy was
associated with higher Message Appraisal ($\beta=.189$,
$p_{\mathrm{FDR}}<.001$) and Source Knowledge ($\beta=.178$,
$p_{\mathrm{FDR}}<.001$). General AI Trust
($\beta=.168$, $p_{\mathrm{FDR}}=.001$) and Objective Financial Literacy
($\beta=.086$, $p_{\mathrm{FDR}}=.038$) were also positively associated
with Source Knowledge. Finally, greater Risk Tolerance was associated with
higher Safety Concern ($\beta=.145$, $p_{\mathrm{FDR}}=.015$) and lower
Source Knowledge ($\beta=-.117$, $p_{\mathrm{FDR}}=.011$).
Targeted exploratory follow-ups found no robust evidence that these
associations differed across communication styles or displayed source
labels after FDR correction (Appendix~\ref{tab:appraisal-style-label-mod}).

\paragraph{Individual differences in Trust formation.}
We next tested whether participant characteristics changed how evaluations
of the advice translated into Trust. For each characteristic, we compared
an additive mixed-effects model with a model jointly adding its
interactions with Message Appraisal, Risk Acknowledgment, Safety Concern,
Source Knowledge, and Overall Quality. These five-degree-of-freedom
likelihood-ratio tests therefore evaluated whether each participant
characteristic altered the evaluation-to-Trust mechanism anywhere across
the five pathways. FDR correction was applied across the seven omnibus
moderator tests.

Three participant characteristics showed significant omnibus moderation
(Table~\ref{tab:trust-moderator-omnibus}): Objective Financial Literacy
($\chi^2(5)=26.45$, $p_{\mathrm{FDR}}<.001$), Human Trust Propensity
($\chi^2(5)=19.95$, $p_{\mathrm{FDR}}=.005$), and General AI Trust
($\chi^2(5)=15.32$, $p_{\mathrm{FDR}}=.021$). The remaining moderator
blocks were not significant after correction.

For significant moderator blocks, we examined the five pathway-specific
interactions as FDR-adjusted follow-up tests. Objective Financial Literacy
localized primarily to the Source Knowledge pathway
($\beta_{\mathrm{int}}=.054$, $p_{\mathrm{FDR}}=.017$).
Simple-slopes analysis showed that Source Knowledge was positively
associated with Trust across literacy levels, but the association became
stronger as Objective Financial Literacy increased:
$\beta=.074$ at $-1$ SD, $\beta=.127$ at the mean, and $\beta=.181$
at $+1$ SD. Thus, greater Objective Financial Literacy was associated with
stronger weighting of perceived Source Knowledge when forming Trust.

HTP localized specifically to Safety Concern
($\beta_{\mathrm{int}}=.056$, $p_{\mathrm{FDR}}=.002$).
Safety Concern was negatively associated with Trust at all levels of HTP,
but this association weakened from $\beta=-.193$ at $-1$ SD to
$\beta=-.136$ at the mean and $\beta=-.080$ at $+1$ SD. Participants
lower in HTP therefore showed a stronger negative association between
perceived safety concerns and Trust.

General AI Trust also showed significant omnibus moderation, but none of
its five pathway-specific interactions survived within-block FDR
correction. Its moderation of Trust formation therefore could not be
reliably localized to a single evaluative dimension.

\paragraph{Individual differences in Reliance.}
We next examined participant-level associations with intended Reliance
using a corresponding sequence of models. General AI Trust was again the
only characteristic showing a robust upstream association with Reliance
($\beta=.227$, $p_{\mathrm{FDR}}<.001$). This association was significantly
reduced after accounting for the four appraisals and Overall Quality
($\beta=.080$, $p_{\mathrm{FDR}}=.003$), but a smaller association remained
after additionally accounting for Trust
($\beta=.053$, $p_{\mathrm{FDR}}=.009$).
None of the other six characteristics showed a robust main association
with Reliance after correction.

Finally, because Trust was the strongest downstream predictor of Reliance,
we tested whether the Trust--Reliance association varied across the seven
participant characteristics. Objective Financial Literacy was the only
significant moderator after FDR correction
($\beta_{\mathrm{int}}=.039$, $p_{\mathrm{FDR}}=.002$).
Trust strongly predicted Reliance at all literacy levels, but the
association increased from $\beta=.562$ at $-1$ SD to $\beta=.601$
at the mean and $\beta=.640$ at $+1$ SD. Thus, Objective Financial
Literacy did not robustly shift overall Reliance, but was associated with
a stronger translation of Trust into intended Reliance.

\paragraph{Moderation of communication style and source attribution.}
As an additional analysis, we tested whether participant characteristics
altered Trust differences across communication styles or displayed source
labels. For each characteristic, communication-style moderation was tested
by comparing the additive Trust model against a model adding the two
Style$\times$Moderator interactions; displayed-label moderation was tested
analogously using the three Label$\times$Moderator interactions. None of
the seven Style or Label omnibus tests survived FDR correction
(Appendix~\ref{tab:style-label-moderation}). General AI Trust showed
nominal evidence of both Style moderation ($p=.027$) and Label moderation
($p=.028$), but neither survived correction
($p_{\mathrm{FDR}}=.192$ and $.198$, respectively). We therefore find no
robust evidence that the measured individual differences systematically
changed participants' relative responses to communication styles or
displayed source identities.

Taken together, these results suggest that individual differences operated
more strongly through the formation and downstream use of Trust than
through differential preferences for particular communication styles or
source labels. General AI Trust primarily distinguished participants'
overall levels of Trust and Reliance, whereas HTP selectively altered the
weight placed on Safety Concern. Objective Financial Literacy selectively
strengthened the association between perceived Source Knowledge and Trust
and further strengthened the relationship between Trust and intended
Reliance.



\subsection{Side-by-Side Comparison of Advices in Ranking Task}
\label{sec:ranking}
\koustuv{keep but needs to be shortened.}

To complement the one-at-a-time evaluations in Task~1, participants then ranked AI-, Expert-, and Online Community (OC)-style advice side by side for a previously unseen financial scenario. Expert-style advice was ranked first by 47.4\% of participants (135/285), compared with 29.1\% for OC advice (83/285) and 23.5\% for AI advice (67/285; Table~\ref{tab:task2_rankings}). A goodness-of-fit test rejected an equal first-choice distribution across the three styles ($\chi^2(2)=26.61$, $p<.001$). Considering the complete rankings, the three communication styles also differed significantly (Friedman $\chi^2(2)=37.16$, $p<.001$, Kendall's $W=.065$). Pairwise Wilcoxon signed-rank tests with Holm correction showed that Expert-style advice was ranked more favorably than both AI-style ($p_{\mathrm{Holm}}<.001$) and OC-style advice ($p_{\mathrm{Holm}}<.001$), whereas AI and OC did not significantly differ ($p_{\mathrm{Holm}}=.733$). Mean ranks were 1.71 for Expert, 2.14 for OC, and 2.15 for AI, where lower values indicate greater preference. Thus, although agreement across participants was modest, Expert-style advice showed a consistent comparative advantage.

Importantly, this preference remained when no source attribution was displayed. Within the Unlabeled condition, 47.8\% of participants ranked Expert-style advice first, compared with 31.5\% for OC and 20.7\% for AI advice. Rankings again differed significantly (Friedman $\chi^2(2)=16.72$, $p<.001$, $W=.091$), with Expert-style advice preferred over both AI ($p_{\mathrm{Holm}}<.001$) and OC ($p_{\mathrm{Holm}}<.001$), while AI and OC did not differ ($p_{\mathrm{Holm}}=.691$). Descriptively, Expert-style advice was ranked first by 53.0\% of participants in the correctly Labeled condition, 47.8\% in the Unlabeled condition, and 40.9\% in the Mislabeled condition. However, a Plackett--Luce rank-choice model found no significant overall Advice Style $\times$ Attribution Arm interaction ($\chi^2(4)=6.65$, $p=.155$). Across arms, Expert-style advice had greater relative preference than AI-style advice (OR$=1.81$, 95\% CI $[1.46,2.25]$, $p<.001$), whereas OC and AI advice did not significantly differ (OR$=.96$, 95\% CI $[.77,1.20]$, $p=.720$). We therefore find evidence for an overall Expert-style preference, but not that the relative ranking of the three styles systematically changed across attribution conditions.

Participants' reported ranking criteria further foregrounded properties of the advice itself. Clear reasoning (65.6\%), ease of reading and understanding (60.0\%), situational relevance (53.3\%), and acknowledgment of risks and uncertainties (50.9\%) were the most frequently selected considerations. In contrast, only 7.0\% explicitly reported that the displayed source influenced their ranking (Figure~\ref{fig:ranking_criteria}). Source influence was reported more frequently in the correctly Labeled condition (15.0\%) than in the Mislabeled (5.4\%) or Unlabeled (0\%) conditions ($\chi^2(2)=17.09$, $p_{\mathrm{FDR}}=.002$); no other ranking criterion differed across attribution arms after FDR correction. These criteria are self-reported and therefore do not identify the causal determinants of ranking, but provide complementary evidence that participants primarily described their comparative judgments in terms of message-level evaluative cues. Nine participants (3.2\%) additionally provided a free-text ``Other'' criterion. Although too few for systematic qualitative analysis, these comments echoed several 
of the experimentally varied communication cues: participants mentioned 
relatability and personability, neutrality of tone, the breadth of considerations 
raised by the advice, and perceived source bias. Two participants instead noted 
that the three recommendations appeared very similar, while one described their 
ranking as a ``gut feeling.'' We treat these responses as illustrative rather than 
as evidence of the prevalence of these considerations. Participants were also generally confident in their rankings ($M=3.68$, $SD=.89$ on a five-point scale; median $=4$), with 61.1\% reporting that they were very or extremely confident. Ranking confidence did not significantly differ across attribution arms (omnibus Wald $\chi^2(2)=2.02$, $p=.365$).

\input{tables/35_ranking_main}






\subsection{Robustness Checks}
\koustuv{move to appendix}

\paragraph{Within- and between-participant variation.}
Because each participant evaluated four advice responses, associations
between appraisals and downstream judgments could partly reflect stable
individual response tendencies. We therefore decomposed each
time-varying predictor into a participant mean (between-participant
variation) and its deviation from that participant's own mean
(within-participant variation), and re-estimated the Quality, Trust, and
Reliance models using both components simultaneously.

The principal evaluation pathway was preserved at the within-participant
level. Message Appraisal ($\beta_W=.329$), Risk Acknowledgment
($\beta_W=.073$), Safety Concern ($\beta_W=-.106$), and Source
Knowledge ($\beta_W=.444$) retained their expected associations with
Overall Quality (all $p\leq.001$). In the Trust model, Message Appraisal
($\beta_W=.147$), Safety Concern ($\beta_W=-.159$), Source Knowledge
($\beta_W=.108$), and Overall Quality ($\beta_W=.573$) remained
significant in the expected directions; Risk Acknowledgment showed a
smaller positive within-participant association
($\beta_W=.048$, $p=.018$). Finally, Trust remained the dominant
within-participant predictor of Reliance
($\beta_W=.533$, $p<.001$), alongside Overall Quality
($\beta_W=.221$), Message Appraisal ($\beta_W=.113$), and Safety
Concern ($\beta_W=-.087$; all $p<.001$).
These results indicate that the observed evaluation pathway cannot be
explained solely by stable differences between participants who
generally rate advice more or less positively.

\paragraph{Alternative Repeated-Measures Estimation.}
As a second robustness check, we re-estimated the core evaluation-pathway
models using generalized estimating equations (GEE) with an exchangeable
working correlation to account for repeated evaluations within
participants. The resulting coefficients closely reproduced the
mixed-effects estimates across Overall Quality, Trust, and Reliance.
For example, the Quality--Trust association was $\beta=.608$ under GEE
(compared with $.607$ in the mixed-effects model), while the
Trust--Reliance association was $\beta=.595$ (compared with $.594$).
The direction and inferential conclusions of the principal pathways were
unchanged. The only exception was the small direct Source
Knowledge--Reliance association, whose coefficient remained similar
($\beta=.048$) but was not statistically distinguishable from zero under
GEE ($p=.084$). Overall, the substantive pathway conclusions were robust
to an alternative treatment of within-participant dependence.

\paragraph{Scenario fixed effects.}
We further examined whether the evaluation pathway depended on our
parameterization of decision context. We replaced the stakes,
uncertainty, and verifiability indicators with fixed effects for each of
the eight scenarios, thereby absorbing stable differences between
individual decision scenarios beyond the three designed context
dimensions. The pathway estimates remained nearly unchanged. For
example, the Message Appraisal--Quality association was $\beta=.320$
(compared with $.325$ in the primary model), the Source
Knowledge--Quality association was $\beta=.491$ (vs.\ $.489$), the
Overall Quality--Trust association was $\beta=.603$ (vs.\ $.607$), and
the Trust--Reliance association was $\beta=.593$ (vs.\ $.594$).
The direction and inferential conclusions of the remaining appraisal
paths were similarly preserved. Thus, the downstream evaluation pathway
was robust to absorbing scenario-specific heterogeneity rather than
representing decision context solely through the three designed
dimensions.

\paragraph{Item-level sensitivity.}
Finally, we examined whether the results depended on aggregating
readability, reasoning clarity, and situational fit into Message
Appraisal, or financial-harm risk and misleadingness into Safety
Concern. We replaced both composites with their constituent items and
re-estimated the Quality, Trust, and Reliance models. Joint Wald tests
showed that the three message-appraisal items remained jointly associated
with Overall Quality ($\chi^2(3)=211.04$, $p<.001$), Trust
($\chi^2(3)=35.79$, $p<.001$), and Reliance
($\chi^2(3)=16.67$, $p<.001$). The two safety-concern items were
likewise jointly associated with Overall Quality
($\chi^2(2)=23.70$, $p<.001$), Trust
($\chi^2(2)=56.55$, $p<.001$), and Reliance
($\chi^2(2)=12.45$, $p=.002$). Moreover, the principal downstream
coefficients were nearly unchanged: Overall Quality predicted Trust at
$\beta=.598$ (vs.\ $.607$ in the primary model), while Overall Quality
and Trust predicted Reliance at $\beta=.208$ and $\beta=.594$
(vs.\ $.206$ and $.594$, respectively). Thus, the principal pathway
results were not dependent on the construction of the two appraisal
composites.
