# Supplementary material for: Trustworthy FinAInce: Unpacking How AI-Mediated Financial Advice is Judged
Source: arXiv:2609.20989 source file (2026-09-21)
Supplement: Supplementary file 4 [file 34_validation_appendix.tex]

\section{Stimulus Validation Details}
\label{app:stimulus_validation_details}

\subsection{Linguistic Analysis of the Constructed Stimuli}

We applied a common preprocessing pipeline to all 24 constructed advice texts. The lexical/style measures were response length, words per sentence, lexical repetition (the normalized proportion of non-unique word tokens), mean word length, Coleman--Liau grade level, sentence-averaged formality, first-person singular language, second-person language, conditional markers, modal verbs, hedging markers, and contractions. Rates are reported per 100 words where indicated. Formality was estimated with the \texttt{s-nlp/roberta-base-formality-ranker} classifier by scoring each sentence and averaging sentence-level formal probabilities within each response. Because the three styles were matched within each of the eight scenarios, we used Friedman tests for omnibus comparisons and applied Benjamini--Hochberg correction across these 12 lexical/style measures. Table~\ref{tab:supp_constructed_linguistic} reports the complete results. CDI was analyzed as an additional LIWC-style summary measure and is shown in the final row; its omnibus test was conducted separately from the 12-measure FDR family.

\begin{table*}[t]
\centering
\caption{Complete linguistic differentiation of the constructed communication styles. Cells report $M$ ($SD$).}
\label{tab:supp_constructed_linguistic}
\scriptsize
\setlength{\tabcolsep}{4pt}
\begin{tabular}{lrrrrr}
\toprule
Measure & AI & Expert & Online Community & $\chi^2(2)$ & $p_{\mathrm{FDR}}$ \\
\midrule
Word count & 173.125 (17.016) & 165.250 (13.036) & 165.625 (14.162) & 7.000 & .0362 \\
Words per sentence & 15.846 (2.238) & 19.203 (1.648) & 13.992 (2.082) & 13.000 & .0037 \\
Lexical repetition & .330 (.026) & .291 (.029) & .296 (.033) & 9.250 & .0147 \\
Mean word length & 5.341 (.166) & 5.251 (.237) & 4.413 (.204) & 12.250 & .0037 \\
Coleman--Liau grade level & 13.668 (1.203) & 13.389 (1.531) & 7.743 (1.228) & 12.250 & .0037 \\
Formality & .824 (.045) & .801 (.060) & .521 (.061) & 13.000 & .0037 \\
First-person singular / 100 words & .000 (.000) & .624 (.390) & 3.664 (2.169) & 15.548 & .0037 \\
Second-person / 100 words & 4.512 (1.535) & 4.649 (1.194) & 2.946 (1.705) & 4.750 & .0930 \\
Conditional markers / 100 words & 2.390 (.475) & 1.171 (1.119) & 1.105 (.700) & 4.750 & .0930 \\
Modal verbs / 100 words & 1.713 (.761) & 2.496 (1.026) & 1.116 (.555) & 7.750 & .0277 \\
Hedging markers / 100 words & 1.590 (1.057) & 2.128 (1.025) & .521 (.582) & 12.250 & .0037 \\
Contractions / 100 words & .000 (.000) & 1.590 (1.507) & 3.581 (.983) & 13.067 & .0037 \\
\midrule
Categorical--Dynamic Index (CDI)$^{\dagger}$ & 27.359 (5.319) & 21.302 (5.042) & 12.028 (5.004) & 14.250 & .0008$^{\dagger}$ \\
\bottomrule
\end{tabular}

\vspace{2pt}
\footnotesize\emph{Note.} Benjamini--Hochberg correction was applied across the 12 lexical/style measures above CDI. $^{\dagger}$CDI was tested separately; the value shown is the unadjusted omnibus $p$-value. CDI was calculated as $30+\mathrm{article}+\mathrm{preposition}-\mathrm{personal\ pronoun}-\mathrm{impersonal\ pronoun}-\mathrm{auxiliary\ verb}-\mathrm{conjunction}-\mathrm{adverb}-\mathrm{negation}$, with LIWC-style category frequencies expressed as percentages. Paired Wilcoxon comparisons for CDI remained significant after FDR correction for AI vs.\ Expert ($p_{\mathrm{FDR}}=.023$), AI vs.\ Online Community ($p_{\mathrm{FDR}}=.012$), and Expert vs.\ Online Community ($p_{\mathrm{FDR}}=.012$).
\end{table*}

\subsection{External Reference-Corpus Validation}

To assess whether the constructed profiles were grounded in source-associated patterns beyond the study stimuli, we assembled a topic-matched external reference corpus containing 72 financial-advice texts: 24 AI responses, 24 professional financial-advice texts, and 24 online-community responses. Each of the eight study topics contributed three reference texts per source category. We applied the same feature-extraction pipeline used for the constructed stimuli, excluding raw response length because the source units differed in genre. For inferential comparisons, the three reference texts within each scenario-by-source cell were averaged first, yielding eight matched AI--Expert--Online Community triplets. We then applied Friedman tests across the eight topic-matched triplets and Benjamini--Hochberg correction across the 12 external-validation features shown in Table~\ref{tab:supp_external_linguistic}.

\begin{table*}[t]
\centering
\caption{Linguistic profiles of the external reference corpus and topic-matched omnibus tests. Cells report $M$ ($SD$) across the 24 texts in each source category.}
\label{tab:supp_external_linguistic}
\scriptsize
\setlength{\tabcolsep}{4pt}
\begin{tabular}{lrrrrr}
\toprule
Measure & AI & Expert & Online Community & $\chi^2(2)$ & $p_{\mathrm{FDR}}$ \\
\midrule
Words per sentence & 24.288 (7.620) & 18.987 (3.355) & 17.931 (6.376) & 6.250 & .0586 \\
Lexical repetition & .376 (.047) & .399 (.038) & .323 (.086) & 5.250 & .0869 \\
Mean word length & 4.958 (.262) & 4.930 (.385) & 4.272 (.295) & 13.000 & .0066 \\
Coleman--Liau grade level & 12.039 (1.967) & 11.449 (2.329) & 7.114 (2.142) & 12.250 & .0066 \\
Formality & .530 (.094) & .733 (.101) & .572 (.168) & 12.250 & .0066 \\
First-person singular / 100 words & .139 (.236) & .587 (1.145) & 1.974 (2.353) & 14.000 & .0066 \\
Second-person / 100 words & .310 (1.193) & 3.525 (1.961) & 5.148 (3.205) & 10.750 & .0111 \\
Conditional markers / 100 words & .959 (.754) & .689 (.623) & 1.324 (.922) & 6.250 & .0586 \\
Modal verbs / 100 words & 1.673 (1.292) & 1.830 (.921) & 1.780 (1.516) & .250 & .8825 \\
Hedging markers / 100 words & .877 (.870) & .726 (.541) & .926 (.973) & .250 & .8825 \\
Contractions / 100 words & 1.145 (1.551) & 1.427 (1.310) & 2.547 (1.315) & 9.250 & .0196 \\
Categorical--Dynamic Index (CDI) & 27.314 (8.510) & 22.924 (7.605) & 12.047 (9.264) & 7.750 & .0356 \\
\bottomrule
\end{tabular}

\vspace{2pt}
\footnotesize\emph{Note.} Omnibus tests were conducted on scenario-by-source cell means (three reference texts averaged within each cell), preserving the eight-topic matched structure. Benjamini--Hochberg correction was applied across the 12 external-validation features in this table. For CDI, FDR-adjusted pairwise comparisons distinguished AI from Online Community ($p_{\mathrm{FDR}}=.035$) and Expert from Online Community ($p_{\mathrm{FDR}}=.035$), while AI and Expert were not statistically distinguishable ($p_{\mathrm{FDR}}=.078$). For formality, Expert differed from both AI and Online Community after within-measure FDR correction ($p_{\mathrm{FDR}}=.012$ for each), whereas AI and Online Community did not differ ($p_{\mathrm{FDR}}=.383$).
\end{table*}

The external corpus therefore supports several broad source-associated differences represented in the constructed manipulation, but not every individual cue. In particular, both corpora showed substantially greater lexical complexity and higher Coleman--Liau grade levels for AI/Expert than for Online Community advice, increasing first-person singular language toward Online Community advice, and increasing contraction use toward Online Community communication. CDI showed especially close correspondence in absolute means and ordering. Formality was more nuanced: the constructed stimuli showed AI and Expert as similarly formal and Online Community as less formal, whereas the external corpus showed Expert as the most formal source and no reliable AI--Online Community difference. Likewise, second-person address, conditional markers, and hedging did not reproduce the same source ordering. These departures reinforce our interpretation of the stimuli as controlled source-associated profiles rather than literal replicas of naturally occurring messages.

\subsection{Semantic Alignment Across Constructed Variants}

We used normalized Sentence-BERT embeddings to assess whether the three stylistic renderings retained scenario-specific semantic content. Table~\ref{tab:supp_semantic_alignment} reports cosine similarity for matched variants from the same scenario and the average similarity between texts from different scenarios. Across all three style pairs, matched similarity was substantially higher than unmatched similarity. We additionally treated each response as a retrieval query against all responses in the comparison style. In each of the 24 directed queries, the highest-similarity response corresponded to the same financial scenario.

\begin{table}[t]
\centering
\caption{Semantic alignment of the constructed communication-style variants.}
\label{tab:supp_semantic_alignment}
\small
\setlength{\tabcolsep}{5pt}
\begin{tabular}{lrrrr}
\toprule
Style pair & Matched $M$ ($SD$) & Unmatched $M$ & $\Delta$ & Top-1 \\
\midrule
AI--Expert & .844 (.035) & .304 & .540 & 8/8 \\
AI--OC & .728 (.107) & .282 & .446 & 8/8 \\
Expert--OC & .798 (.054) & .293 & .505 & 8/8 \\
\bottomrule
\end{tabular}

\vspace{2pt}
\footnotesize\emph{Note.} $\Delta$ is the difference between mean same-scenario and different-scenario cosine similarity. Top-1 reports whether the nearest response in the comparison style corresponded to the same scenario; the three directed comparisons comprise 24 retrieval queries in total.
\end{table}

\subsection{Independent Human Validation}

Three independent annotators completed a blind stimulus audit. For the source-style check, annotators saw the 24 advice texts without intended-source labels, classified the source each response most resembled, rated four communication characteristics on five-point scales, and reported confidence. For content parity, annotators compared the three unlabeled responses within each scenario and judged whether they shared the same recommendation direction, scenario-specific facts, and core financial rationale, as well as whether any response introduced potentially material additional information.

\begin{table}[t]
\centering
\caption{Summary of independent human validation.}
\label{tab:supp_human_validation}
\small
\setlength{\tabcolsep}{5pt}
\begin{tabular}{p{0.48\columnwidth}r}
\toprule
Validation criterion & Result \\
\midrule
\multicolumn{2}{l}{\emph{Blind source-style recognition}} \\
Correct individual classifications & 66/72 (91.7\%) \\
Correct majority classification & 24/24 (100\%) \\
Unanimously correct stimuli & 18/24 (75.0\%) \\
Fleiss' $\kappa$ & .749 \\
\midrule
\multicolumn{2}{l}{\emph{Content-parity judgments}} \\
Same recommendation direction & 23/24 (95.8\%); majority 8/8 \\
Same scenario-specific facts & 24/24 (100\%); majority 8/8 \\
Same core financial rationale & 23/24 (95.8\%); majority 8/8 \\
Potentially material extra information & 15/24 (62.5\%); majority 5/8 \\
\bottomrule
\end{tabular}

\vspace{2pt}
\footnotesize\emph{Note.} Each content-parity judgment corresponds to one annotator evaluating one scenario triplet ($3$ annotators $\times$ $8$ scenarios $=24$ judgments). All six individual source-classification errors were confusions between AI and Expert; all 24 judgments for Online Community stimuli were correct. Among responses explicitly flagged for additional information, 14 of 16 flagged responses were Online Community variants, typically because of additional anecdotal evidence. A separate contradiction item showed an apparent polarity-interpretation inconsistency for one annotator and is therefore not used as a primary parity metric; majority judgment nevertheless indicated no contradiction in all eight scenario triplets.
\end{table}

\begin{table}[t]
\centering
\caption{Human ratings of communication characteristics by intended style. Values are $M$ ($SD$) on five-point scales.}
\label{tab:supp_style_ratings}
\small
\setlength{\tabcolsep}{4pt}
\begin{tabular}{lrrr}
\toprule
Characteristic & AI & Expert & Online Community \\
\midrule
Professional / measured & 4.50 (.66) & 4.58 (.88) & 2.08 (.58) \\
Analytical / impersonal & 4.75 (.44) & 4.46 (.51) & 1.96 (1.00) \\
Conversational / peer-like & 1.46 (.66) & 1.88 (.74) & 4.50 (.78) \\
Personal experience / anecdotal & 1.00 (.00) & 1.04 (.20) & 4.92 (.28) \\
\bottomrule
\end{tabular}

\vspace{2pt}
\footnotesize\emph{Note.} Each style is represented by 24 ratings ($8$ stimuli $\times$ $3$ annotators). These ratings are treated as a descriptive manipulation check rather than as population-level estimates of how the source categories are perceived.
\end{table}

\subsection{Validation Summary}

Taken together, the validation checks support three narrower claims needed for the experimental design. First, the constructed variants were linguistically and perceptually distinguishable as source-associated communication styles. Second, the variants retained the same core financial decision, recommendation direction, scenario facts, and financial rationale, while Online Community responses sometimes added source-characteristic anecdotal support. Third, several broad linguistic profiles in the constructed stimuli were also present in the external reference corpus, although not every individual stylistic cue generalized. Accordingly, throughout the paper we interpret the manipulation as varying controlled source-associated communication profiles while holding the common substantive decision backbone as constant as practicable.

% ---------------------------------------------------------------------------
% CITATION TODOs BEFORE CAMERA-READY
% 1. Coleman & Liau (1975) for the Coleman--Liau Index.
% 2. Pennebaker et al. (2014) for the CDI formulation; confirm and cite the
%    exact provenance/version of the LIWC-style dictionary used.
% 3. Babakov et al. (2023) / the associated formality-model source for
%    s-nlp/roberta-base-formality-ranker; optionally cite Saha et al. (2026)
%    as the methodological precedent for this linguistic-validation battery.
% 4. Reimers & Gurevych (2019) for Sentence-BERT and Song et al. (2020) for MPNet.
% 5. Benjamini & Hochberg (1995) for FDR correction and Fleiss (1971) for kappa.
% ---------------------------------------------------------------------------
