# Supplementary material for: Trustworthy FinAInce: Unpacking How AI-Mediated Financial Advice is Judged
Source: arXiv:2609.20989 source file (2026-09-21)
Supplement: Supplementary file 5 [file 36_ranking_supplementary.tex]

\subsection{Additional Analyses of the Comparative Ranking Task}
\label{app:task2}

\subsubsection{Rank-Distribution Tests}

The overall preference pattern remained robust when we considered the complete ranking, not just the first-ranked response. A Friedman test indicated that rank distributions differed across AI-, Expert-, and OC-style advice ($\chi^2(2)=37.16$, $p<.001$, Kendall's $W=.065$). Holm-adjusted pairwise Wilcoxon signed-rank tests indicated that Expert-style advice was ranked more favorably than AI- and OC-style advice, whereas AI and OC advice did not significantly differ (Table~\ref{tab:supp_pairwise_ranking}).

We repeated these comparisons in the Unlabeled condition to examine preferences without explicit source attribution. The omnibus difference remained significant ($\chi^2(2)=16.72$, $p<.001$, $W=.091$), with Expert-style advice again ranked more favorably than both AI and OC advice. AI and OC advice did not significantly differ.

\begin{table}[t]
\caption{Pairwise Wilcoxon signed-rank comparisons of Task~2 rankings. Holm-adjusted $p$-values correct for the three pairwise comparisons within each analysis. Lower mean rank indicates greater preference.}
\label{tab:supp_pairwise_ranking}
\centering
\small
\begin{tabular}{llrrrr}
\toprule
Sample & Contrast & Mean Rank A & Mean Rank B & $W$ & $p_{\mathrm{Holm}}$ \\
\midrule
Overall
    & Expert vs.\ AI & 1.705 & 2.154 & 13110.0 & $<.001$ \\
    & Expert vs.\ OC & 1.705 & 2.140 & 13477.0 & $<.001$ \\
    & AI vs.\ OC     & 2.154 & 2.140 & 19921.0 & .733 \\
\midrule
Unlabeled
    & Expert vs.\ AI & 1.652 & 2.185 & 1192.0 & $<.001$ \\
    & Expert vs.\ OC & 1.652 & 2.163 & 1274.0 & $<.001$ \\
    & AI vs.\ OC     & 2.185 & 2.163 & 2040.5 & .691 \\
\bottomrule
\end{tabular}

\vspace{2pt}
\footnotesize
\textit{Note.} Overall Friedman test: $\chi^2(2)=37.16$, $p<.001$, Kendall's $W=.065$. Unlabeled-condition Friedman test: $\chi^2(2)=16.72$, $p<.001$, $W=.091$.
\end{table}


\subsubsection{Rank-Choice Models and Attribution Conditions}

We additionally modeled the complete rankings using Plackett--Luce rank-choice models, with AI-style advice as the reference alternative. Across all participants, Expert-style advice had greater relative preference than AI-style advice (OR$=1.81$, 95\% CI $[1.46,2.25]$, $p<.001$), whereas OC-style advice did not differ from AI-style advice (OR$=.96$, 95\% CI $[.77,1.20]$, $p=.720$).

Separate models within each attribution condition showed a significant Expert-over-AI preference in the Unlabeled and correctly Labeled conditions, but not in the Mislabeled condition (Table~\ref{tab:supp_plackett}). However, these descriptive differences across arms should not be interpreted as evidence that mislabeling altered preference: allowing source preferences to vary across attribution arms did not significantly improve model fit relative to a common-preference model (likelihood-ratio $\chi^2(4)=6.65$, $p=.155$).

\begin{table}[t]
\caption{Plackett--Luce models of comparative advice rankings overall and within each attribution condition. AI-style advice is the reference alternative.}
\label{tab:supp_plackett}
\centering
\small
\begin{tabular}{llrrr}
\toprule
Sample & Contrast & OR & 95\% CI & $p$ \\
\midrule
Overall
    & Expert vs.\ AI & 1.81 & [1.46, 2.25] & $<.001$ \\
    & OC vs.\ AI     & 0.96 & [0.77, 1.20] & .720 \\
\midrule
Unlabeled
    & Expert vs.\ AI & 2.03 & [1.39, 2.98] & $<.001$ \\
    & OC vs.\ AI     & 0.91 & [0.61, 1.35] & .630 \\
\midrule
Labeled
    & Expert vs.\ AI & 2.30 & [1.57, 3.37] & $<.001$ \\
    & OC vs.\ AI     & 1.02 & [0.70, 1.48] & .930 \\
\midrule
Mislabeled
    & Expert vs.\ AI & 1.28 & [0.88, 1.86] & .199 \\
    & OC vs.\ AI     & 0.95 & [0.65, 1.39] & .795 \\
\bottomrule
\end{tabular}

\vspace{2pt}
\footnotesize
\textit{Note.} Odds ratios represent relative preference in the rank-choice model. The Advice Style $\times$ Attribution Arm interaction did not significantly improve model fit, $\chi^2(4)=6.65$, $p=.155$.
\end{table}


\subsubsection{Reported Ranking Criteria}

Participants most frequently reported clear reasoning, readability, situational relevance, and acknowledgment of risks and uncertainties as considerations informing their rankings (Table~\ref{tab:supp_ranking_reasons}). Across the ten reported criteria, only explicit source influence differed significantly across attribution conditions after Benjamini--Hochberg correction ($\chi^2(2)=17.09$, $p_{\mathrm{FDR}}=.002$). Source influence was reported by 15.0\% of participants in the correctly Labeled condition, 5.4\% in the Mislabeled condition, and none in the Unlabeled condition. No other criterion showed a robust attribution-arm difference.

\begin{table*}[t]
\caption{Self-reported criteria used in the comparative ranking task. Participants could select multiple criteria. Attribution-arm differences were tested using $3\times2$ chi-square tests with Benjamini--Hochberg FDR correction across the ten criteria.}
\label{tab:supp_ranking_reasons}
\centering
\small
\begin{tabular}{lrrrrrr}
\toprule
Criterion
& Overall
& Labeled
& Unlabeled
& Mislabeled
& $\chi^2(2)$
& $p_{\mathrm{FDR}}$ \\
\midrule
Clear reasoning
& 187 (65.6\%) & 63.0\% & 64.1\% & 69.9\% & 1.15 & .759 \\

Easy to read and understand
& 171 (60.0\%) & 60.0\% & 60.9\% & 59.1\% & 0.06 & .972 \\

Relevant to the situation
& 152 (53.3\%) & 58.0\% & 47.8\% & 53.8\% & 2.00 & .759 \\

Acknowledges risks and uncertainties
& 145 (50.9\%) & 52.0\% & 54.3\% & 46.2\% & 1.30 & .759 \\

Reliable overall
& 127 (44.6\%) & 49.0\% & 40.2\% & 44.1\% & 1.51 & .759 \\

Aligned with own thinking/preferences
& 114 (40.0\%) & 34.0\% & 39.1\% & 47.3\% & 3.60 & .759 \\

Safe to follow
& 106 (37.2\%) & 41.0\% & 35.9\% & 34.4\% & 1.00 & .759 \\

Unlikely to be misunderstood/cause a poor decision
& 65 (22.8\%) & 24.0\% & 26.1\% & 18.3\% & 1.73 & .759 \\

Source influenced my ranking
& 20 (7.0\%) & 15.0\% & 0.0\% & 5.4\% & \textbf{17.09} & \textbf{.002} \\

Other
& 9 (3.2\%) & 4.0\% & 3.3\% & 2.2\% & 0.54 & .847 \\
\bottomrule
\end{tabular}
\end{table*}


\paragraph{Free-text ranking criteria.}
Participants who selected ``Other'' could additionally describe a consideration 
not represented by the predefined ranking criteria. Nine participants (3.2\% of 
the sample) provided such a response. We reviewed these comments descriptively 
rather than conducting formal qualitative coding because of the small and 
self-selected response set. Several comments referred to communication qualities 
that complement the predefined criteria. Participants described advice as 
``personable/relatable,'' valued a relatable example that made consequences easier 
to connect to their own situation, and commented on the neutrality or general 
presentation of the advice. One participant valued that a recommendation introduced 
additional considerations, such as a future home purchase, while another explicitly 
described AI as ``least biased.'' Two participants indicated that the three 
recommendations were highly similar, and one attributed the ranking to a ``gut 
feeling.'' These responses provide illustrative evidence that comparative judgments 
could also incorporate tone, experiential connection, perceived neutrality, and 
broader decision framing beyond the predefined response categories.

\begin{table}[t]
\caption{Illustrative responses from participants who used the free-text ``Other''
field when describing their Task~2 ranking criteria. Responses are presented
without participant identifiers and are not treated as a formal qualitative
coding analysis.}
\label{tab:supp_ranking_freetext}
\centering
\small
\begin{tabular}{p{0.28\linewidth}p{0.64\linewidth}}
\toprule
Illustrative consideration & Example response \\
\midrule

Relatability / experiential connection
& ``Was personable/relatable.'' \\

Relatable examples
& ``The advice included a relatable example that illustrated the potential
impact of decisions, making it easier to connect with and apply to my own
situation.'' \\

Tone / neutrality
& ``I thought the tone was most neutral in the 1st choice, which I found to
be optimal.'' \\

Breadth of considerations
& ``Adds additional things to consider like home purchase.'' \\

Perceived source bias
& ``The AI is least biased.'' \\

Low differentiation
& ``Honestly they were all pretty much the same.'' \\
& ``All fairly similar.'' \\

Intuitive judgment
& ``Gut feeling.'' \\

General presentation
& ``I liked the way it presented its advice.'' \\

\bottomrule
\end{tabular}
\end{table}
